# Supplementary material for: Satellite Selection for In-Band Coexistence of Dense LEO Networks
Source: arXiv:2503.15262 source file (2025-03-19)
Supplement: Supplementary file 1 [file sec-appendix.tex]

\vspace{-0.2cm}
\appendix

% \section{Lagrangian relaxation}

\setcounter{equation}{32}
The dual function $g(\lambda, \mu, \boldsymbol\nu)$ is obtained by maximizing the Lagrangian over $\bX^t$ subject to the assignment constraints: 
%\begin{align}
%	g(\lambda_\sfu, \mu) &= \max_\vx g(\vx; \lambda_\sfu, \mu), \quad \forall \sfu, \\
%	\st & \sum_m x_{m,n} = 1, \\
%	& x_{m,n} \in \braces{0,1}.
%\end{align}
\begin{subequations}
\begin{align}
	g(\lambda, & \mu, \boldsymbol\nu) = \max_{\bX^t} g(\bX^t; \lambda, \mu, \boldsymbol\nu) \\
	\st & \sum_m x_{m,n}^t \leq 1, \\
	&\,\, x_{m,n}^t \in \braces{0,1}.
\end{align}
\end{subequations}
%\subsubsection{Subproblems:} Given Lagrangian multiplier $\lambda_{m,n}$ and $\mu_m$, the Lagrangian dual problem leads to the decomposed subproblem for each cluster $n$ as follows: 
% \subsection{Subproblems}
\setcounter{equation}{35}
Given Lagrangian multipliers $\lambda$, $\mu$ and $\boldsymbol\nu$, the maximization over $x_{m,n}^t$ can be decomposed for each $n$ as 
     \eqref{eq:sp_1}. %-$\eqref{eq:sp_3}. 
Therefore, for each $n$, we aim to find the optimal $m_n^{\opt}$ satisfying \eqref{eq:m_star} and 
\begin{align}
	x_{m,n}^t = \begin{cases}
		1, \qquad \text{if } m = m\opt_n, \\
		0, \qquad \text{otherwise}.
	\end{cases}
\end{align}
Then we compute the dual function $g(\lambda, \mu, \boldsymbol\nu)$ by plugging in the selected $x_{m,n}^t$, then we use subgadient methods to solve the dual problem 
$\min_{\lambda \geq 0, \mu\geq 0, \boldsymbol\nu \geq \boldsymbol{0}} g(\lambda, \mu, \boldsymbol\nu)$.
% \begin{align}
%     \min_{\lambda \geq 0, \mu, \boldsymbol\nu \geq 0} g(\lambda, \mu, \boldsymbol\nu).
% \end{align}

% \subsection{Subgradient Iterations} 
In Lagrangian relaxation methods, subgradient iterative techniques can be used to update the set of Lagrange multipliers. 
This begins by initializing the Lagrangian multipliers as $\lambda^{(0)} \geq 0$, $\mu^{(0)}\geq 0$, and $\boldsymbol\nu^{(0)}\geq\boldsymbol{0}$. 
The subgradients $s^{(k)}(\lambda)$, $s^{(k)}(\mu)$, and $s^{(k)}(\boldsymbol\nu)$ are then calculated as
\begin{align}
	&s^{(k)}(\lambda) %= \frac{\partial{L(\bX, \lambda)}}{\partial{\lambda}} 
	=  \ttminrth - \max_{\sfu\in\mathcal{U}}\sum_{m=1}^{\nums}\sum_{n=1}^{\numg}c_{m,n}\cdot x_{m,n}^{t(k)},\\
     &s^{(k)}(\mu) = \minrth^{\mathrm{max}} -\!\! \max_{\sfu\in\mathcal{U}, \tau \in \mathcal{T}}\sum_{m=1}^{\nums}\sum_{n=1}^{\numg} \minr^\tau(\sfu, \vp_\sfu; \vs_m, \vg_n) \cdot x_{m,n}^{t(k)},\\
   &s^{(k)}(\nu_m) =  1 -  \sum_{n=1}^{\numg} x_{m,n}^{t(k)}, \,\, \forall m,
\end{align}
where $x_{m,n}^{t(k)}$ represents the optimal solution of the relaxed problem for the current $\lambda^{(k)}$, $\mu^{(k)}$, and $\boldsymbol\nu^{(k)}$. 
The update rules for $\lambda$, $\mu$ and $\boldsymbol\nu$ %with the subgradient method 
are
\begin{align}
&	\lambda^{(k)} = \max\braces{0,\,\,\lambda^{(k-1)} + \alpha^{(k)} \cdot s^{(k)}(\lambda}, \\
&	\mu^{(k)} = \max\braces{\boldsymbol{0},\,\,\mu^{(k-1)} + \beta^{(k)} \cdot s^{(k)}(\mu)},\\
&	\boldsymbol\nu^{(k)} = \max\braces{0,\,\,\boldsymbol\nu^{(k-1)} + \gamma^{(k)} \cdot s^{(k)}(\boldsymbol\nu)}, %\forall m,
\end{align}
where $\alpha^{(k)}$, $\beta^{(k)}$ and  $\gamma^{(k)}$ are the step sizes % or learning rates 
at iteration $k$. 

\setcounter{equation}{33}
\begin{figure*}[t]
    \vspace{-0.2cm}
	% ensure that we have normalsize text
	\normalsize
	% Store the current equation number.
	%	\setcounter{mytempeqncnt}{\value{equation}}
	%\setcounter{equation}{4}
	% Set the equation number to one less than the one
	% desired for the first equation here.
	% The value here will have to changed if equations
	% are added or removed prior to the place these
	% equations are referenced in the main text.
	%	\setcounter{equation}{4}
	\begin{align}
	 \max_{\bX^t} &\sum_{m=1}^{N_s}\braces{ c_{m,n}^t-\lambda \cdot \max_{\sfu\in\mathcal{U}} \tminrTht(\sfu, \vp_\sfu; \vs_m, \vg_n) -\mu \cdot \max_{\sfu\in\mathcal{U}, \tau \in \mathcal{T}} \minr^\tau(\sfu, \vp_\sfu; \vs_m, \vg_n) - \nu_m}\cdot x_{m,n}^t. \label{eq:sp_1}
		% \st & x_{m,n} \in \braces{0,1},\,\,\forall m, \\
		%&\sum_{m=1}^{N_s} x_{m,n} \leq 1. \label{eq:sp_3}
	\end{align}
	
	% Restore the current equation number.
	%	\setcounter{equation}{\value{mytempeqncnt}}
	%	\setcounter{equation}{5}
	% IEEE uses as a separator
	\hrulefill
	% The spacer can be tweaked to stop underfull vboxes.
	%\vspace*{4pt}
    \vspace{-0.3cm}
\end{figure*}
\begin{figure*}[t]
    \vspace{-0.2cm}
	% ensure that we have normalsize text
	\normalsize
	% Store the current equation number.
	%	\setcounter{mytempeqncnt}{\value{equation}}
	%\setcounter{equation}{4}
	% Set the equation number to one less than the one
	% desired for the first equation here.
	% The value here will have to changed if equations
	% are added or removed prior to the place these
	% equations are referenced in the main text.
	%	\setcounter{equation}{4}
		
	\begin{align}
		m\opt_n = \argmax_m \sum_{m=1}^{\nums}\braces{c_{m,n}^t-\lambda \cdot \max_{\sfu\in\mathcal{U}} \tminrTht(\sfu, \vp_\sfu; \vs_m, \vg_n)  - \mu \cdot \max_{\sfu\in\mathcal{U}, \tau \in \mathcal{T}} \minr^\tau(\sfu, \vp_\sfu; \vs_m, \vg_n)  - \nu_m}.%\cdot x_{m,n}, 
    %,\forall n, 
    \label{eq:m_star}
	\end{align}
	% Restore the current equation number.
	%	\setcounter{equation}{\value{mytempeqncnt}}
	%	\setcounter{equation}{5}
	% IEEE uses as a separator
	\hrulefill
	% The spacer can be tweaked to stop underfull vboxes.
	%\vspace*{4pt}
    \vspace{-0.3cm}
\end{figure*}

\vspace{-0.12cm}
\section*{Acknowledgments}

We thank Arun Ghosh, Michael Hicks, Anil Rao, and Vikram Chandrasekhar from Amazon's Project Kuiper for their %valuable 
discussions and feedback on our methodology and results.
\vspace{-0.1cm}
